# Supplementary material for: Evolution of magnetic interactions in a pressure-induced Jahn-Teller driven magnetic dimensionality switch
Source: arXiv:1304.5403 ancillary file (2013-04-19)
Supplement: Supplementary file 1 [file Supplamental_Info.pdf]

# SUPPLEMENTAL INFORMATION

## Evolution of magnetic interactions in a pressure-induced Jahn-Teller driven magnetic dimensionality switch

S. Ghannadzadeh,[1,*] J. S. Möller,[1,†] P. A. Goddard,[1] T. Lancaster,[2] F. Xiao,[2] S. J. Blundell,[1] A. Maisuradze,[3] R. Khasanov,[3] J. L. Manson,[4] S. W. Tozer,[5] D. Graf,[5] and J. A. Schlueter[6]

[1]*Clarendon Laboratory, Department of Physics, University of Oxford, Parks Road, Oxford, OX1 3PU, UK*
[2]*Department of Physics, Durham University, South Road, Durham, DH1 3LE, UK*
[3]*Laboratory for Muon Spin Spectroscopy, Paul Scherrer Institut, CH-5232 Villigen PSI, Switzerland*
[4]*Department of Chemistry and Biochemistry, Eastern Washington University, Cheney, WA 99004, USA*
[5]*National High Magnetic Field Laboratory, Florida State University, Tallahassee, FL 32310, USA*
[6]*Materials Science Division, Argonne National Laboratory, Argonne, IL 60439, USA*

### EXCHANGE ENERGY

We use the single-$J$ convention, such that in a system with just two exchange-coupled spin–1/2 spins, the energy difference between the $S = 0$ singlet and $S = 1$ triplet at zero magnetic field is $k_{\rm B}J$.

### MUON EXPERIMENT

The positron decay asymmetry is defined as $A(t) = (N_{\rm F} - \alpha N_{\rm B})/(N_{\rm F} + \alpha N_{\rm B})$ where $N_{\rm F}$ ($N_{\rm B}$) is the number of positrons observed in detectors forward (backward) of the initial muon spin direction and $\alpha$ is an experimental calibration constant.

The data taken at ambient pressure and 4.8 kbar were fitted to

$$\begin{aligned} A(t) =& A_1 e^{-\lambda_1 t}\cos(2\pi\nu_1 t + \phi_1) \\ &+ A_2 e^{-\lambda_2 t}\cos(2\pi\nu_2 t + \phi_2) \\ &+ A_3 e^{-\lambda_3 t}\cos(2\pi\nu_3 t + \phi_3) + A_4 e^{-\lambda_4 t} + A_{\rm b}(t), \end{aligned}$$

where $\nu$ are the dominant oscillation frequencies due to long-range magnetic order of the sample, $\phi$ are constant phases, and the exponential terms account for residual magnetic dynamics in the sample. The last term accounts for the signal from muons stopped in the pressure cell itself, and is well described by $A_{\rm b}(t) = \frac{1}{3}A_{\rm cell} + \frac{2}{3}A_{\rm cell}\exp(-\frac{1}{2}\Delta^2 t^2)(1 - \Delta^2 t^2)$, where $\Delta$ is the width of the internal field distribution in the cell and $A_{\rm cell}$ is the amplitude of the signal from the muons stopped in the cell. For all fits, the ratios $A_1 : A_2 : A_3$ and $\nu_1 : \nu_2 : \nu_3$ were fixed to be $4 : 2 : 1$ and $1 : 0.65 : 0.55$ respectively, as in Ref. [1].

Similarly, the data taken at $\geq 11.2$ kbar were fitted to

$$A(t) = A_5 e^{-\lambda_5 t}\cos(2\pi\nu_5 t) + A_6 e^{-\lambda_6 t} + A_{\rm b}(t).$$

The data taken at 10.5 kbar showed a phase separation between the Q2D and Q1D phases, and were fitted to

$$\begin{aligned} A(t) =& A_1 e^{-\lambda_1 t}\cos(2\pi\nu_1 t + \phi_1) \\ &+ A_2 e^{-\lambda_2 t}\cos(2\pi\nu_2 t + \phi_2) \\ &+ A_3 e^{-\lambda_3 t}\cos(2\pi\nu_3 t + \phi_3) + A_4 e^{-\lambda_4 t} \\ &+ A_5 e^{-\lambda_5 t}\cos(2\pi\nu_5 t) + A_6 e^{-\lambda_6 t} + A_{\rm b}(t), \end{aligned}$$

where $A_5$ and $A_6$ were fixed to zero above the Q1D ordering transition around 0.5 K.

### PRESSURE CALIBRATION FOR $\mu^+$SR MEASUREMENTS

A Cu-Be piston-cylinder cell was used for the measurements at 1 and 10.5 kbar, while a cell made from MP35 alloy was used for 4.8, 11.2, 14.8, and 22.5 kbar measurements. In the Cu-Be (MP35) cell approximately

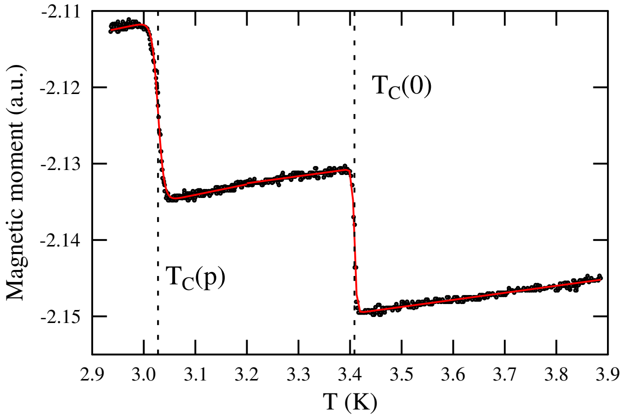


FIG. S1. AC susceptibility measurement of the superconducting transition temperature in indium platelets placed inside the pressure cell at 10.5 kbar (lower transition) and outside of the cell (higher transition). The red line is a fit to a step function with a finite width, which was used to estimate the non-hydrostaticity across the indium platelet and the error on the pressure.

| | Pressure (kbar) | $B_c$ (K) | $J$ (K) | $T_N$ (K) | $J_\perp$ (mK) |
|---|---|---|---|---|---|
| Magnetization | 0.001 | 28.1(3) | 11.4(3) | - | - |
| | 5.9(2) | 24.8(3) | 10.0(2) | - | - |
| | 9.1(2) [a] | 23.4(3) | 9.5(2) | - | - |
| | 9.1(2) [a] | 7.9(1) | 5.5(1) | - | - |
| | 12.9(2) | 8.3(1) | 5.9(1) | - | - |
| | 15.6(2) | 8.9(1) | 6.3(2) | - | - |
| | 20(1) | 9.4(1) | 6.6(2) | - | - |
| $\mu^+$SR | 0.001 | - | 11.4(3) [b] | 2.59(1) [c] | 5(1) |
| | 1.0(5) | - | 11.1(2) [b] | 2.48(1) | 4.2(9) |
| | 4.8(1) | - | 10.3(2) [b] | 2.11(3) | 1.5(4) |
| | 10.5(2) [a] | - | 9.1(2) [b] | 2.15(3) | 6(2) |
| | 10.5(2) [a] | - | 5.7(2) [b] | 0.5(1) | 280(80) |
| | 11.2(2) | - | 5.7(1) [b] | 0.535(5) | 290(3) |
| | 14.8(3) | - | 6.1(2) [b] | 0.570(6) | 308(4) |
| | 22.5(5) | - | 6.9(2) [b] | 0.628(8) | 339(5) |

[a] Assuming phase separation.
[b] Found through interpolation of $J$ from the magnetization data.
[c] From Manson *et al.* [1].

TABLE S1. Top: The critical field $B_c$ and the associated primary exchange energy $J$ deduced from magnetization measurements. Bottom: The long range ordering temperature $T_N$ from $\mu^+$SR measurements. $J_\perp$ was calculated using empirical equations from Quantum Monte-Carlo simulations [2].

50% (30%) of the signal originated from the sample. Daphne oil 7373 was used as the pressure medium. Apart from the 1 kbar measurement, the pressure inside the cell was determined by measuring the shift of superconducting transition temperature $T_C$ of a platelet of indium placed inside the cell with respect to the superconducting transition of an identical platelet placed outside the cell. The pressure inside the cell is then given by $P = (T_C(0) - T_C(p))/0.0364$, where temperatures are in K and the pressure is in kbar. $T_C$ was measured using a separate AC susceptibility setup. An example measurement is shown in Fig. S1. The indium platelets were approximately 10% of the sample size. The width of the transition is an approximate measure of the nonhydrostaticity of the pressure across the indium platelet and was used to estimate the errors on the measured pressures.

## ZERO-FIELD MOMENT IN THE Q2D PHASE

As explained in the paper, we calculate a zero-field moment of $0.46 \pm 0.01\,\mu_B$ in the Q1D phase. The structural changes occurring during the Q2D to Q1D dimensionality switch only have a small effect on the F–Cu distances [3, 4]. A previous experiment [1] has shown that muons form F–$\mu$ bound states in the low-pressure Q2D phase. If all muons localize in F–$\mu$ bound states in both phases, the muon position relative to the magnetic Cu ions would therefore not change significantly between the two phases and any change in the measured precession frequency $\nu(T=0)$ would be due to a change in the Cu moment. Note that this is consistent with the observation that $\nu(T=0)$ is constant within the Q1D phase, despite the changes in $T_N$. Assuming that, due to the increase in quantum fluctuations with a reduction in dimensionality, the frequencies from the Q2D phase broaden to yield the frequency of the Q1D phase, then the corresponding reduction in Cu moment size from Q2D to Q1D phase is approximately 50% (taking the average of the frequencies in the Q2D phase as reference). Hence one would expect nearly the full Cu moment of $1\,\mu_B$ in the Q2D phase.

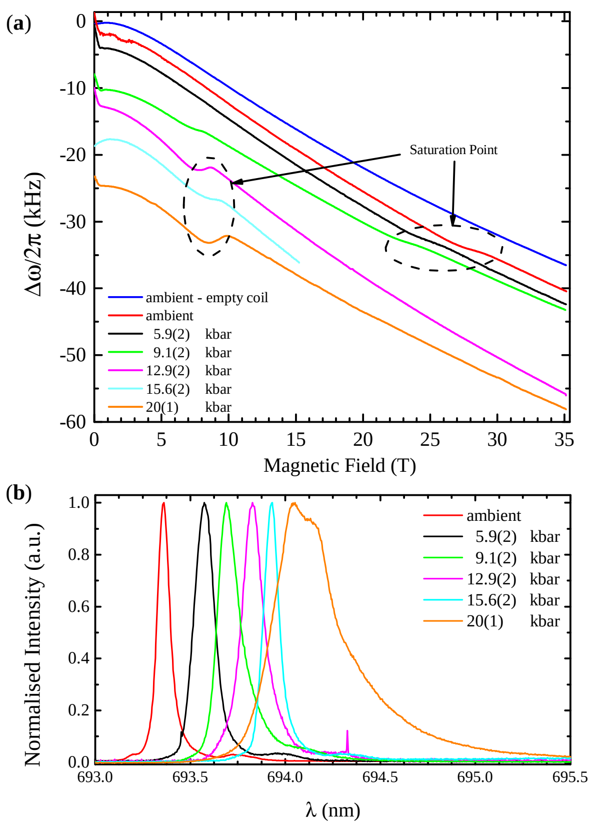


FIG. S2. (a) Change in the resonance frequency of the susceptometer as a function of magnetic field, for $CuF_2(H_2O)_2$(pyz), across a range of pressures. The data have been shifted vertically for clarity. Also in blue is an empty coil measurement at ambient pressure. (b) $R_1$ laser fluorescence response of ruby chips inside the pressure cell, at $T \approx 1.4$ K.

## MAGNETIZATION

The magnetization was measured using a Proximity Detector Oscillator Dynamic Susceptometer, which has been proved to be an effective method of measuring the dynamic susceptibility $\chi = \mathrm{d}M/\mathrm{d}H$, and hence through integration, the magnetization [5]. This susceptometer consists of an external Proximity Detector Oscillator, which is coupled to a resonator coil containing the sample

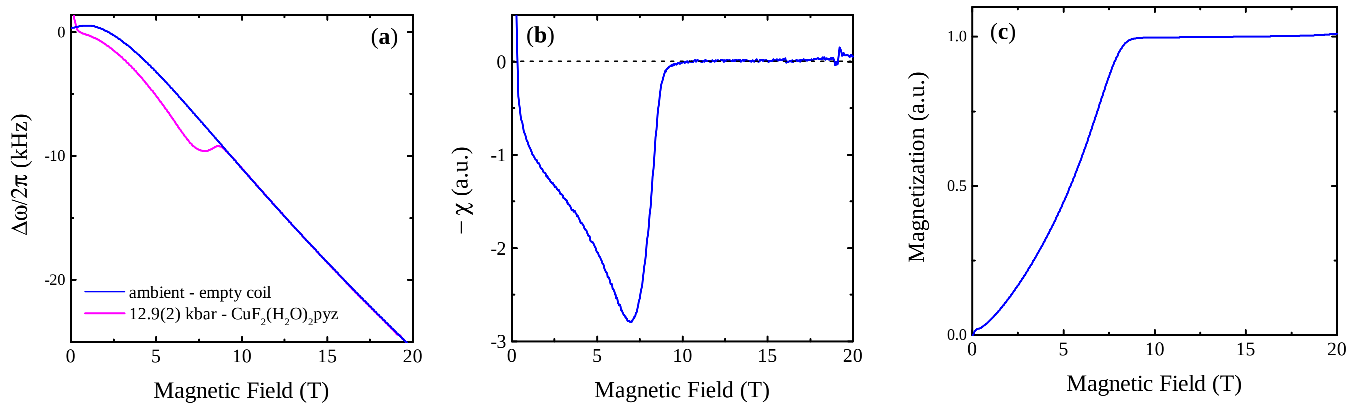


FIG. S3. (a) Resonance frequency for an empty resonator coil (rescaled by a factor of 1.2), and for one with $CuF_2(H_2O)_2$(pyz) single crystals at 12.9 kbar and $T = 1.4$ K. Also included is (b) the resulting magnetic susceptibility, which was integrated to give (c) the magnetization.

to be measured. As detailed in Ref. [5], in an insulating sample, the change in the resonator frequency $\omega$ upon the application of a magnetic field consists of a magnetoresistive background originating from the resonator coil, and an inductive term from the sample itself, via

$$\Delta\omega = -a\Delta\chi - b\Delta R_0, \qquad \text{(S1)}$$

where $\Delta R_0$ is the magnetoresistive background of the resonator coil, $\Delta\chi(H) = \chi(H) - \chi_0$ is the change in the dynamic susceptibility upon application of magnetic field, and $a$, $b$ and $\chi_0$ are constants. Thus, the dynamic susceptibility can be found through subtraction of an empty coil background measurement, since

$$\chi(H) \propto \Delta\omega_{\text{background}} - \Delta\omega_{\text{with sample}} + \chi_0. \qquad \text{(S2)}$$

Once the background is removed from the data, the magnetization can be found by integration. The dynamic susceptibility is zero after saturation, and so $\chi_0$ is equal to the difference of the sample and background frequencies above the saturation point.

The relatively large sample space provided by the piston cylinder cell allowed for a multi-turn coil of 8 turns of 75 µm thick Cu wire, with a coil diameter of 1 mm and with the field parallel to the crystal $a$-axis. In order to characterize any changes in the magnetoresistive background of the system as a function of pressure, empty pressure cells were loaded and tested at various pressures in a Quantum Design Physical Properties Measurement System [6], in fields of up to 16 T. It was found that, other than a slight rescaling, applied pressure induced no features in the magnetoresistance background.

The frequency response of the system, for samples of $CuF_2(H_2O)_2$(pyz) across a range of pressures, is given in Fig. S2. Also shown is an empty coil background measurement at ambient pressure. At each pressure, the magnetoresistive background was deduced by choosing an appropriate value for $b$, such that the background measurement matched the sample coil response above the saturation point; for example see Fig. S3. The magnetization was then found by subtraction of the scaled background data, and integration of the residual according to Equation S2.

## PRESSURE CALIBRATION AND HYDROSTATICITY IN SINGLE CRYSTAL MAGNETIZATION MEASUREMENTS

A 50:50 mix of Fluorinert 70:77 was used as the pressure medium for all magnetization measurements, except a later measurement at 15.6 kbar in which we used Daphne 7474. The pressure was measured in situ at 1.4 K (2 K for the 15.6 kbar run) through the $R_1$-line fluorescence of small ruby chips placed within the pressure cell, with the signal being brought out on an aluminum clad fiber optic. Any applied pressure causes a linear wavelength shift (0.0365 nm/kbar) in the $R_1$ peak position, as shown in Fig. S2(b), which can be used to calibrate the pressure [7]. The pressure errors given in Table S1 are determined by the uncertainty in the measured $R_1$ wavelength shift. The ruby chip calibrants used were approximately 10% of the sample size.

The hydrostaticity can be estimated through analysis of the fluorescence peak sharpness [8, 9]. As shown in Fig. S2(b), we observe no major increase in the peak width with applied pressures up to 15.6 kbar, an indication of good hydrostatic conditions. This is further supported by the fact that there is little difference between the Fluorinert and the Daphne 7474 measurements (Daphne 7474 is known to be hydrostatic up to ≈ 37 kbar at room temperature [10]). We do observe a broadening of the peak at 20 kbar, which can be an indication of some non-hydrostaticity.

To prevent any crystal desolvation over time, fresh samples were grown shortly before the experiments, and

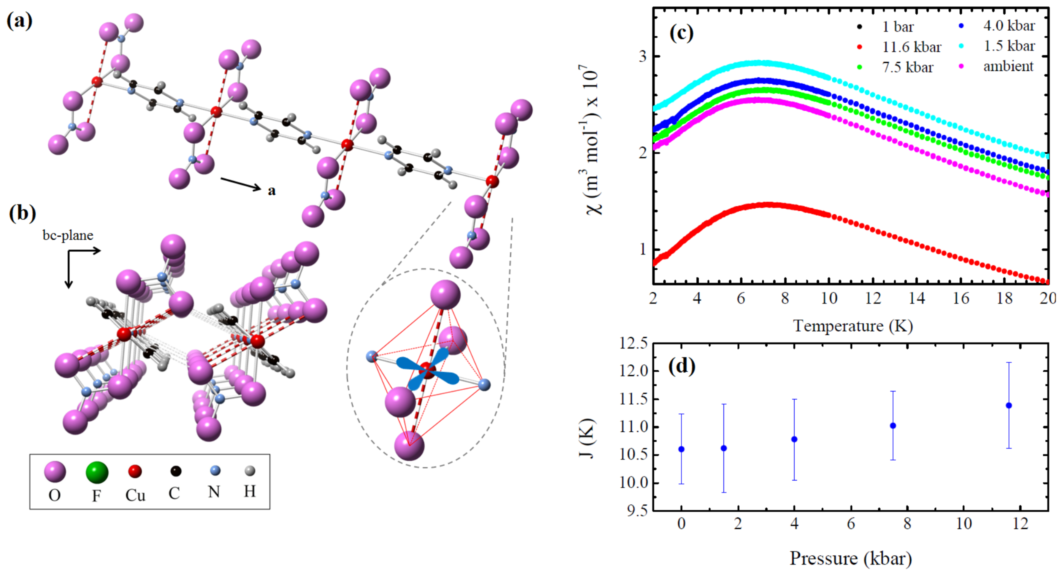


FIG. S4. Crystal structure of $Cu(NO_3)_2$(pyz) at ambient pressure, along the (a) $a$-axis, and (b) the $bc$-plane. The red striped bonds represent the JT-axis. The zoomed-in region shows the JT octahedron, together with one possible representation of the magnetic orbitals. (c) Low field (0.1 T) susceptibility measurement of $Cu(NO_3)_2$(pyz) across a range of pressures, with the field parallel to the $a$-axis. (d) A rough approximation of $J$, deduced from the position of the low-field susceptibility peaks.

were kept in solvent until needed. The single crystals were examined upon release of pressure at the end of the experiment, and were found to be unaffected by the applied pressure, further indicating good hydrostatic conditions and absence of any major uniaxial stress.

For the pressure at which the phase separation is seen (9.1 kbar), we can estimate an upper bound on the non-hydrostaticity by looking at the increase in the peak width with respect to an ambient pressure measurement, via $\Delta P = (\text{FWHM}(9.1\,\text{kbar}) - \text{FWHM}(\text{ambient}))\,/(0.0365 \times 2.4)$. This gives an upper bound of $\pm 0.7$ kbar at 9.1 kbar.

## LOW-FIELD MAGNETIC SUSCEPTIBILITY

For a spin–1/2 Heisenberg antiferromagnet, it is possible to deduce a rough estimate of the exchange energy $J$ from the position of the short-range ordering peak in the low-field magnetic susceptibility via

$$k_B T_\chi^{\max} = aJ, \tag{S3}$$

where $a = 0.641$ for a Q1D antiferromagnet [11], or $a = 0.94$ for a Q2D system [12]. From the work of Halder *et al.* [3], this gives $J \approx 10.6$ K at ambient pressure, and $J \approx 5.6$ K at 11.6 kbar, in good agreement with our findings. This estimate is based on measurements made (a) over a wide range of temperatures, and (b) above the long-range ordering temperature $T_N$, whereas our magnetization measurements are done at a set temperature which is below, or in the vicinity of, $T_N$.

Note that the magnetization saturation field $B_c$ is well resolved within the Q1D phase, despite the measurement temperature 1.4 K being above, but close to, $T_N$. This is due to significant short range antiferromagnetic correlations in the vicinity of the onset of long range ordering at $T_N$.

## CU(NO$_3$)$_2$(PYZ)

$Cu(NO_3)_2$(pyz) has a structure very similar to that of $CuF_2(H_2O)_2$(pyz), consisting of Cu–pyz–Cu chains along the $a$-axis, with the Cu-atoms joined together in the plane perpendicular to the chain direction by $NO_3$ bonds, as shown in Figs. S4(a,b). The Cu atoms sit within a distorted octahedral, surrounded by Cu–N and Cu–O ligands. At ambient pressure this material is a Q1D antiferromagnet ($J = 10.6$ K, $T_N = 0.107$ K) [13, 14], with the magnetic orbitals lying within the chain direction.

Pressure measurements were performed on powder samples of $Cu(NO_3)_2$(pyz) using a Quantum Design Magnetic Properties Measurement System [6]. Pressure was achieved by means of a piston cylinder cell, and was calibrated by using a Sn standard.

Low-field (0.1 T) susceptibility measurements as a function of temperature were performed in a range of pressures upto 11.6 kbar, as is shown in Fig. S4(c). The broad peak in susceptibility is due to short range antiferromagnetic ordering above $T_N$. We can estimate the primary exchange energy $J$ via Eqn. S3, as shown in Fig. S4(d). We observe a gradual increase in $J$ with applied pressure at a rate of $67 \pm 6$ mK/kbar. However, unlike

$CuF_2(H_2O)_2$(pyz), we do not detect a modification of the magnetic dimensionality with pressure.

* s.ghannadzadeh1@physics.ox.ac.uk
† j.moeller1@physics.ox.ac.uk for $\mu^+$SR details.

[1] J. L. Manson *et al.*, Chem. Mater. **20**, 7408 (2008).
[2] C. Yasuda *et al.*, Phys. Rev. Lett. **94**, 217201 (2005).
[3] G. J. Halder *et al.*, Angew. Chem. Int. Ed. **50**, 419 (2011).
[4] A. Prescimone *et al.*, Angew. Chem. Int. Ed. **51**, 7490 (2012).
[5] S. Ghannadzadeh *et al.*, Rev. Sci. Instrum. **82**, 113902 (2011).
[6] Qunatum Design USA, www.qdusa.com.
[7] G. J. Piermarini *et al.*, J. Appl. Phys. **46**, 2774 (1975).
[8] Y. Shu-Jie *et al.*, Chin. Phys. Lett. **26**, 096202 (2009).
[9] G. J. Piermarini *et al.*, J. Appl. Phys. **44**, 5377 (1973).
[10] K. Murata *et al.*, Rev. Sci. Instrum. **79**, 085101 (2008).
[11] D. C. Johnston *et al.*, Phys. Rev. B **61**, 9558 (2000).
[12] M. Lines, J. Phys. Chem. Solids **31**, 101 (1970).
[13] P. R. Hammar *et al.*, Phys. Rev. B **59**, 1008 (1999).
[14] T. Lancaster *et al.*, Phys. Rev. B **73**, 020410 (2006).
